# Supplementary material for: A Morton-Type Space-Filling Curve for Pyramid Subdivision and Hybrid Adaptive Mesh Refinement
Source: arXiv:2602.20887 source file (2026-05-22)
Supplement: Supplementary file 1 [file supplement.pdf]

# SUPPLEMENTARY MATERIALS: FORMULAS AND `Ghost` RUNTIME

DAVID KNAPP, JOHANNES HOLKE, THOMAS SPENKE, AND CARSTEN BURSTEDDE

**SM1. Uniform refinement of a root pyramid.** The formula for the number of descendants of a root pyramid at a given level $\ell$ derives from the following recursion,

$$P(\ell+1) = 4 \cdot 2^{3\ell} + 6P(\ell), \qquad \text{where} \qquad P(0) = 1. \tag{SM1.1}$$

If we expand it and simplify, we obtain the following result,

$$\begin{aligned} P(\ell) &= 4\left(6^0 2^{3(\ell-1)} + 6^1 2^{3(\ell-2)} + \ldots + 6^{\ell-1}2^0\right) + 6^\ell \\ &= 4 \cdot 8^{\ell-1} \sum_{k=0}^{\ell-1} \left(\frac{3}{4}\right)^k + 6^\ell = 4 \cdot 8^{\ell-1} \frac{1-(3/4)^\ell}{1-3/4} + 6^\ell \\ &= 2 \cdot 8^\ell - 6^\ell. \end{aligned} \tag{SM1.2}$$

It is easily verified using induction.

**SM2. Performance results of the `Ghost` algorithm.** We display strong scaling results for the ghost algorithm running our largest experiment in Table SM2.1. Weak scaling results follow in Table SM2.2.

| Procs | elems / proc | avg. ghosts/proc | ghost time | runtime | |
|---|---|---|---|---|---|
| | | Pyramid | | per elem | per ghost |
| 4096 | 18.470e6 | 254K | 2.477s | 1.341e-7 | 9.751e-6 |
| 8192 | 9.235e6 | 169K | 1.482s | 1.604e-7 | 8.769e-6 |
| 16K | 4.618e6 | 111K | 1.029s | 2.228e-7 | 9.270e-6 |
| 32K | 2.309e6 | 75K | 0.652s | 2.707e-7 | 8.333e-6 |
| | | Tetrahedron | | per elem | per ghost |
| 4096 | 18.874e6 | 274K | 1.408s | 7.490e-8 | 5.140e-6 |
| 8192 | 9.437e6 | 164K | 0.723s | 7.661e-8 | 4.441e-6 |
| 16K | 4.719e6 | 104K | 0.455s | 9.516e-8 | 4.375e-6 |
| 32K | 2.359e6 | 70K | 0.347s | 1.471e-7 | 4.957e-6 |
| | | Hexahedron | | per elem | per ghost |
| 4096 | 18.874e6 | 230K | 1.312s | 6.951e-8 | 5.704e-6 |
| 8192 | 9.437e6 | 156K | 0.865s | 9.071e-8 | 5.487e-6 |
| 16K | 4.719e6 | 99K | 0.537s | 1.138e-7 | 5.424e-6 |
| 32K | 2.359e6 | 59K | 0.320s | 1.356e-7 | 5.423e-6 |
| | | Prism | | per elem | per ghost |
| 4096 | 18.874e6 | 348K | 2.517s | 1.334e-7 | 7.232e-6 |
| 8192 | 9.437e6 | 194K | 1.265s | 1.340e-7 | 6.521e-6 |
| 16K | 4.719e6 | 138K | 0.843s | 1.786e-7 | 6.109e-6 |
| 32K | 2.359e6 | 90K | 0.614s | 2.602e-7 | 6.822e-6 |

TABLE SM2.1

*The strong scaling and parallel efficiency of the ghost algorithm for the largest configuration of the element benchmark.*

| procs | $l$ | elems/proc | avg. ghosts/proc | ghost time | runtime | |
|---|---|---|---|---|---|---|
| | | Pyramid | | | per elem | per ghost |
| 64 | 7 | 2.246e6 | 50823 | 0.546s | 2.431e-7 | 1.0743e-5 |
| 512 | 8 | 2.272e6 | 64757 | 0.609s | 2.680e-7 | 9.404e-6 |
| 4096 | 9 | 2.292e6 | 72065 | 0.651s | 2.840e-7 | 9.033e-6 |
| 32K | 10 | 2.308e6 | 75245 | 0.652s | 2.825e-7 | 8.665e-6 |
| | | Tetrahedron | | | per elem | per ghost |
| 64 | 8 | 2.359e6 | 55551 | 0.335s | 1.420e-7 | 6.030e-6 |
| 512 | 9 | 2.359e6 | 64131 | 0.343s | 1.454e-7 | 5.348e-6 |
| 4096 | 10 | 2.359e6 | 68431 | 0.346s | 1.467e-7 | 5.056e-6 |
| 32K | 11 | 2.359e6 | 70583 | 0.347s | 1.491e-7 | 4.916e-6 |
| | | Hexahedron | | | per elem | per ghost |
| 64 | 8 | 2.359e6 | 46080 | 0.314s | 1.331e-7 | 6.814e-6 |
| 512 | 9 | 2.359e6 | 53760 | 0.318s | 1.348e-7 | 5.915e-6 |
| 4096 | 10 | 2.359e6 | 57600 | 0.318s | 1.348e-7 | 5.521e-6 |
| 32K | 11 | 2.359e6 | 59520 | 0.320s | 1.357e-7 | 5.379e-6 |
| | | Prism | | | per elem | per ghost |
| 64 | 8 | 2.359e6 | 71640 | 0.609s | 2.58e-6 | 7.971e-6 |
| 512 | 9 | 2.359e6 | 81876 | 0.611s | 2.59e-6 | 7.463e-6 |
| 4096 | 10 | 2.359e6 | 86994 | 0.613s | 2.60e-6 | 7.046e-6 |
| 32K | 11 | 2.359e6 | 89553 | 0.614s | 2.602e-6 | 6.856e-6 |

TABLE SM2.2

*The weak scaling and parallel efficiency of the ghost algorithm for the largest configuration of the element benchmark.*
